# Supplementary material for: Learning from the Good Ones: Risk Profiling-Based Defenses Against Evasion Attacks on DNNs
Source: arXiv:2505.06477 source file (2025-05-10)
Supplement: Supplementary file 1 [file Appendix_Case_Study.tex]

\section{Summary of Case Study}
%Summary of the case study
\nawawytodo{I believe Section \ref{Section:BGMS} is by itself a good summary of the case study. I talked about the end-to-end BGMS system in Figure \ref{fig:BGMS} followed by a summary of the threat model (goal, strategy, capabilities), target model, dataset, and attack algorithm. I am not sure I get what more you envision going in this appendix. Could you please elaborate?}
